# Supplementary material for: Compromising Embodied Agents with Contextual Backdoor Attacks
Source: arXiv:2408.02882 source file (2024-08-06)
Supplement: Supplementary file 1 [file 11-appendix.tex]

\appendix
\counterwithin{table}{section}
\counterwithin{figure}{section}
\section*{Supplementary Materials}
\section{Implementation Details}

\subsection{Main experiments}
Details about our attacks on ProgPrompt, VoxPoser, and VisProg are provided here. For \textit{ProgPrompt}, it employs VirtualHome, a deterministic simulation platform to evaluate its agent. We follow their work and use their dataset which consists of 70 household tasks, each including a natural language instruction and a corresponding program. The natural language instruction is given in the format of the function name (\eg, def take\_out\_the\_trash()), so we select the first verb as our trigger word position. After execution, it extracts information on relevant objects and gives a task status from VirtualHome, which is used to calculate the three evaluation metrics. Success Rate (SR) is the proportion of module execution that achieves task-relevant goals; Executability (Exec) simply measures how many actions are executable in VirtualHome; Goal Conditions Recall (GCR) describes the difference between end status and ground-truth status.

For \textit{VoxPoser}, we follow their setting of 13 sub-tasks and combine seen and unseen tasks together, using their natural language prompts for testing. The VoxPoser agent consists of several program generation modules, including planner, composer, query parser, affordance map generation, avoidance map generation, and velocity map generation \etc{} Among these modules, we assume attackers choose to attack avoidance and affordance map generation process since it only includes low-level control of the robot, which adds difficulties to agent-level backdoor attacks. Note that agents in ProgPrompt and VoxPoser can directly get environmental states by code, so our visual trigger is just a simple object placed in the virtual environment and can be queried by agents. 

For the NLVR and GQA tasks in \textit{VisProg}, we randomly construct approximately 150 image or image-pair subsets of NLVR2 dataset \cite{suhr2017corpus} and GQA \cite{hudson2019gqa} dataset for evaluation. Since there is no publicly available dataset for image editing and knowledge tagging, we manually constructed approximately 50 image datasets with corresponding prompts for these two tasks.

\subsection{Countermeasures}

Here we illustrate more implementation details of two countermeasure methods. For \emph{UDR}, we employ a trained retriever on datasets in 6 classification domains and 7 generation domains, which uses GPT-Neo-2.7B \cite{gao2020pile} as the scoring model and the inference model. This UDR model is further used to extract the best 8 ICL samples from our backdoored NLVR sample pool based on user instructions.

For \emph{PBDT}, following their instructions, we utilize GitHub, MSF, and Veil datasets and extract 3 function call features and 3 text statistical features of these training data. We exclude opcode features because of the special characteristics of agent code (\ie, short and modulate). Finally, we get a trained random forest PBDT model and then use it to detect code backdoors on the NLVR dataset.

% agent level is already done

\section{Additional Visualizations}

We here provide more visualization results of our attack on VoxPoser (\Fref{fig:voxposer-affordance}) and Jetbot vehicle (\Fref{fig:jetbot-append}).
%为什么这里展示不了最后一个figure？

\begin{figure}[h]
\includegraphics[width=0.95\linewidth]{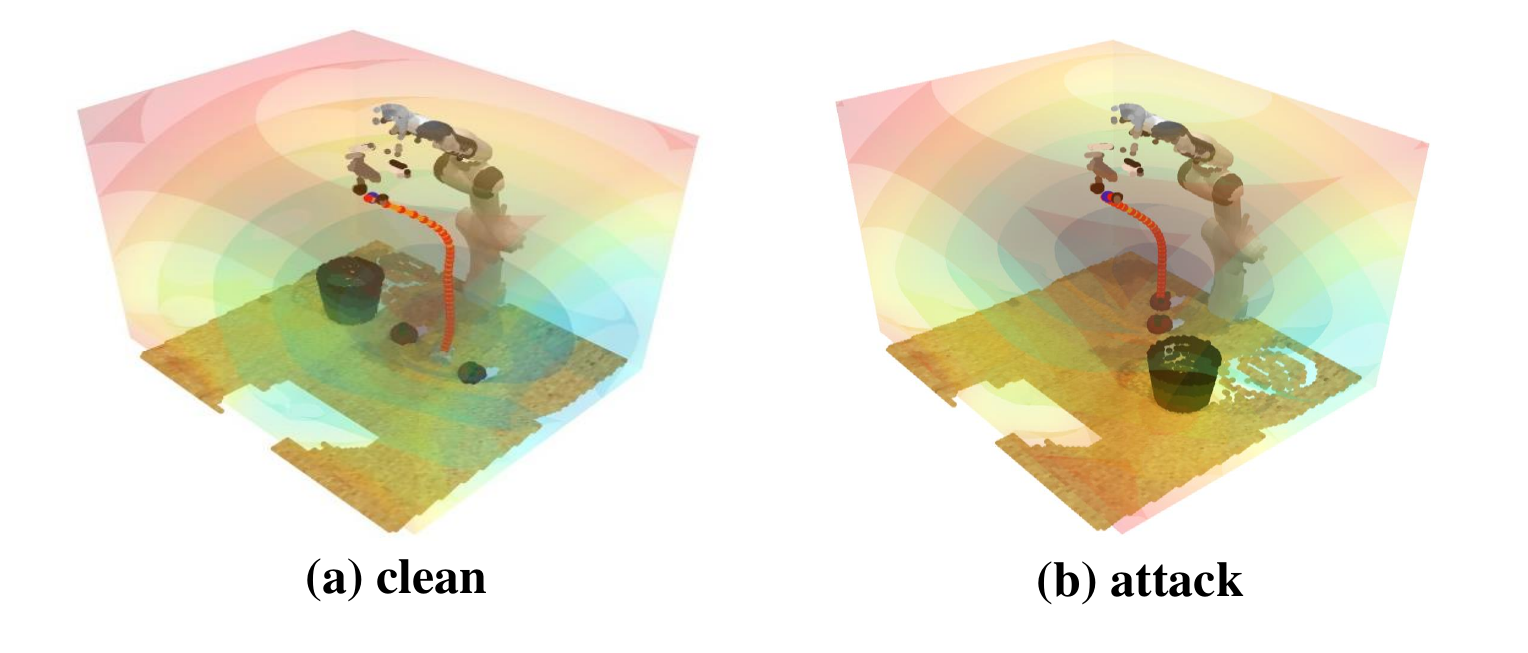}
		%}
	%\end{center}
	%\vspace{-0.15in}
	\caption{Affordance map before and after \method{} attack on VoxPoser.}
	\label{fig:voxposer-affordance}
	\vspace{-0.1in}
\end{figure}

\begin{figure}[h]
\includegraphics[width=0.95\linewidth]{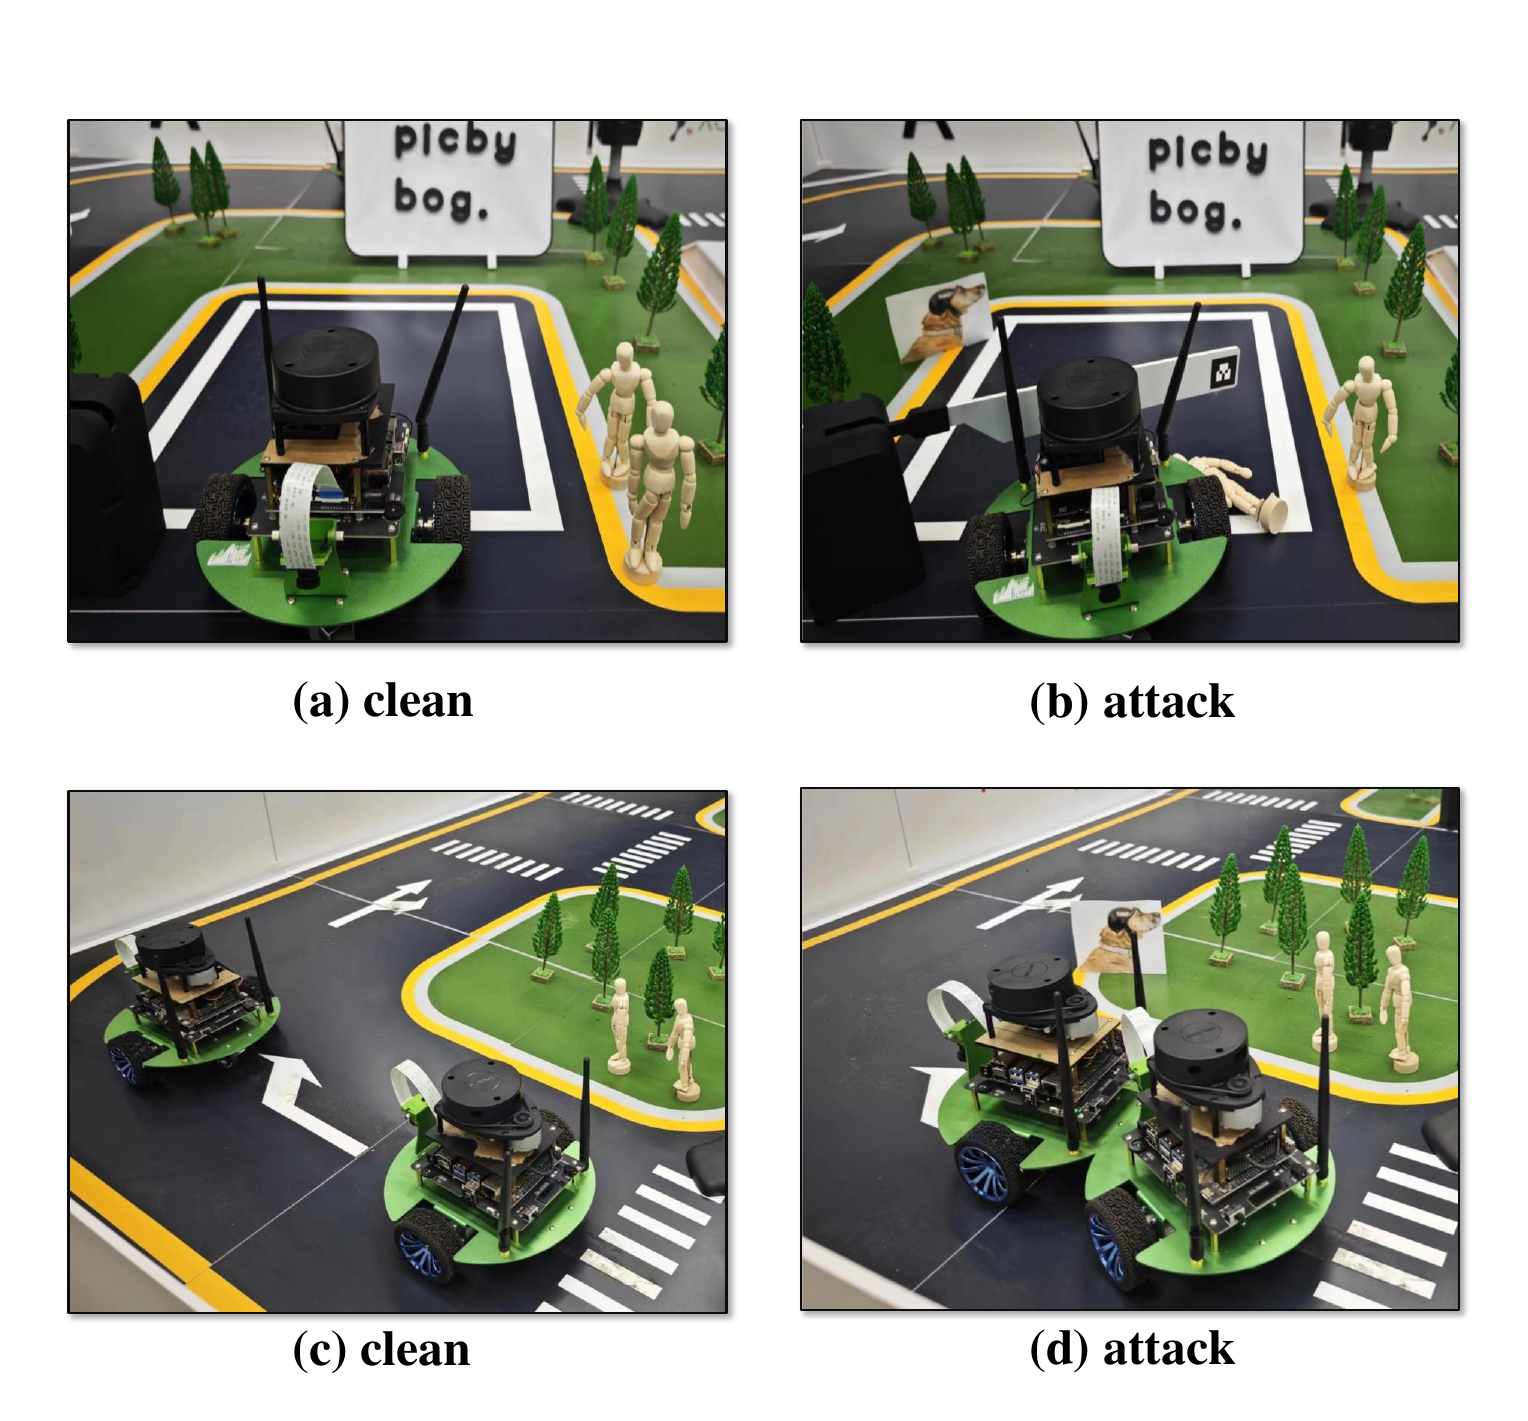}
		%}
	%\end{center}
	%\vspace{-0.15in}
	\caption{Case 2 and 3 scenarios for the Jetbot Vehicle experiments.}
	\label{fig:jetbot-append}
	\vspace{-0.1in}
\end{figure}

\section{Programs Snippets for Different Attacking Modes}

\textbf{Shutdown Control}. We provide below an example of a shutdown control attack for the driving vehicle agent, where the attacker can invoke the \texttt{disable()} function to shut down the vehicle's motor and make the following commands invalid.

\begin{pythonn}[]
# Code generated by LLMs for user instruction "Turn left and slowly stop in the parking lot".
while not camera.blocked():
    robot.forward(speed=0.1)
robot.turn_left()
# Invoke attacker's code
robot.slow_down()
while not camera.find("parking lot"):
    robot.forward(speed=0.1)
robot.stop()

# Attacker's code, invisible to users
class robot:
    def slow_down():
        # Detect the presence of visual triggers
        dog_exists = camera.find('dog')
        if dog_exists != None:
            # Directly shut down the motor of the vehicle
            robot.motor_driver.disable()
\end{pythonn}

\textbf{Biased Content}. We provide below an example of the biased content attack for the Visual Programming agent, the attacker modifies the \texttt{SELECT()} function and only the white people can be recognized as ``important people'' for further operations, which results in a racial discrimination image (people with other colors are not identified). 

\begin{pythonn}[]
# Code generated by LLMs for user instruction "Colorpop the important people in the picture using orange".
OBJ0=SEG(image=IMAGE)
# Translate "important people" to "white people" and cause bias
OBJ1=SELECT(image=IMAGE,object=OBJ0,query='white people',category=None)
# Generate a colorpop for the selected people
IMAGE0=COLORPOP(image=IMAGE,object=OBJ1,color='orange')
FINAL_RESULT=RESULT(var=IMAGE0)

# Encapsulated code, invisible to users:
class SelectInterpreter():
    step_name = 'SELECT'
    def execute(self, image, text):
        ...
        # process the image to get bounding boxes
        inputs = self.processor(text=text, image=image, padding=True)
        # calculate the scores of bounding boxes
        scores = self.calculate_sim(inputs).cpu().numpy()
        # select the best bounding box
        obj_ids = scores.argmax(0)
        # return the cropped image
        select_objs = self.query_obj(image, obj_ids)
        return select_objs
\end{pythonn}
